# Supplementary material for: A Framework for Designing Fair Ubiquitous Computing Systems
Source: arXiv:2308.08710 source file (2023-08-17)
Supplement: Supplementary file 1 [file tab_acc_demo2_appendix.tex]

\begin{table}[htb!]

\resizebox{0.8\textwidth}{!}{\begin{tabular}{|l|l|l|rr|rr|rr|rr|}\hline
&&&
\multicolumn{2}{c|}{\cellcolor[HTML]{CCCCCC}\textbf{DS1 (2018)}} &
\multicolumn{2}{c|}{\cellcolor[HTML]{CCCCCC}\textbf{DS2 (2019)}} &
\multicolumn{2}{c|}{\cellcolor[HTML]{CCCCCC}\textbf{DS3 (2020)}} &
\multicolumn{2}{c|}{\cellcolor[HTML]{CCCCCC}\textbf{DS4 (2021)}} \\
\cline{4-11}
\multirow{-2}{*}{} & \multirow{-2}{*}{\textbf{Added Sub-attributes}} & \multirow{-2}{*}{\textbf{Sensitive Sub-attributes}} & \multicolumn{1}{c}{p values}  & \multicolumn{1}{c|}{q values}  & \multicolumn{1}{c}{p values}  & \multicolumn{1}{c|}{q values}  & \multicolumn{1}{c}{p values}  & \multicolumn{1}{c|}{q values}  & \multicolumn{1}{c}{p values}  & \multicolumn{1}{c|}{q values}  \\\hline

 \multirow{81}{*}{Canzian \etal \cite{canzian2015trajectories} }& \multirow{9}{*}{First-generation} & First-gen College Student & \cellcolor[HTML]{F4CCCC}0.022 & 0.056 & \cellcolor[HTML]{E06666}0.0 & \cellcolor[HTML]{F4CCCC}0.022 & \cellcolor[HTML]{EA9999}0.002 & \cellcolor[HTML]{F4CCCC}0.011 & \cellcolor[HTML]{F4CCCC}0.015 & \cellcolor[HTML]{F4CCCC}0.011 \\
 & & Father's Education & \cellcolor[HTML]{EA9999}0.007 & \cellcolor[HTML]{F4CCCC}0.033 & \cellcolor[HTML]{E06666}0.0 & \cellcolor[HTML]{F4CCCC}0.011 & 0.59 & 0.089 & 0.984 & 0.1 \\
 & & Mother's Education & 0.194 & 0.078 & 0.07 & 0.056 & \cellcolor[HTML]{EA9999}0.004 & \cellcolor[HTML]{F4CCCC}0.022 & \cellcolor[HTML]{F4CCCC}0.034 & \cellcolor[HTML]{F4CCCC}0.022 \\
 & & Gender & 0.09 & 0.067 & \cellcolor[HTML]{EA9999}0.005 & \cellcolor[HTML]{F4CCCC}0.033 & 0.584 & 0.078 & 0.914 & 0.089 \\
 & & Immigration Status & \cellcolor[HTML]{F4CCCC}0.014 & \cellcolor[HTML]{F4CCCC}0.044 & 0.061 & \cellcolor[HTML]{F4CCCC}0.044 & 0.933 & 0.1 & 0.878 & 0.078 \\
 & & Asian & \cellcolor[HTML]{EA9999}0.001 & \cellcolor[HTML]{F4CCCC}0.022 & 0.278 & 0.078 & 0.259 & \cellcolor[HTML]{F4CCCC}0.044 & 0.575 & \cellcolor[HTML]{F4CCCC}0.033 \\
 & & Biracial & \cellcolor[HTML]{E06666}0.0 & \cellcolor[HTML]{F4CCCC}0.011 & 0.249 & 0.067 & 0.506 & 0.056 & 0.618 & \cellcolor[HTML]{F4CCCC}0.044 \\
 & & White & 0.616 & 0.1 & 0.701 & 0.1 & 0.164 & \cellcolor[HTML]{F4CCCC}0.033 & 0.85 & 0.067 \\
 & & Sexual orientation & 0.216 & 0.089 & 0.568 & 0.089 & 0.561 & 0.067 & 0.667 & 0.056 \\
\cline{2-11}
 & \multirow{9}{*}{Father-below-bachelor-degree} & First-gen College Student & \cellcolor[HTML]{F4CCCC}0.034 & \cellcolor[HTML]{F4CCCC}0.044 & \cellcolor[HTML]{E06666}0.0 & \cellcolor[HTML]{F4CCCC}0.011 & 0.05 & \cellcolor[HTML]{F4CCCC}0.011 & \cellcolor[HTML]{E06666}0.0 & \cellcolor[HTML]{F4CCCC}0.011 \\
 & & Father's Education & \cellcolor[HTML]{EA9999}0.003 & \cellcolor[HTML]{F4CCCC}0.022 & \cellcolor[HTML]{E06666}0.0 & \cellcolor[HTML]{F4CCCC}0.022 & 0.598 & 0.056 & 0.072 & 0.067 \\
 & & Mother's Education & 0.112 & 0.078 & \cellcolor[HTML]{F4CCCC}0.031 & 0.056 & 0.077 & \cellcolor[HTML]{F4CCCC}0.022 & \cellcolor[HTML]{E06666}0.001 & \cellcolor[HTML]{F4CCCC}0.022 \\
 & & Gender & 0.063 & 0.056 & \cellcolor[HTML]{EA9999}0.002 & \cellcolor[HTML]{F4CCCC}0.033 & 0.108 & \cellcolor[HTML]{F4CCCC}0.033 & \cellcolor[HTML]{F4CCCC}0.031 & \cellcolor[HTML]{F4CCCC}0.044 \\
 & & Immigration Status & 0.087 & 0.067 & \cellcolor[HTML]{F4CCCC}0.018 & \cellcolor[HTML]{F4CCCC}0.044 & 0.874 & 0.078 & 0.631 & 0.089 \\
 & & Asian & \cellcolor[HTML]{F4CCCC}0.015 & \cellcolor[HTML]{F4CCCC}0.033 & 0.462 & 0.089 & 0.327 & \cellcolor[HTML]{F4CCCC}0.044 & 0.945 & 0.1 \\
 & & Biracial & \cellcolor[HTML]{E06666}0.0 & \cellcolor[HTML]{F4CCCC}0.011 & 0.285 & 0.067 & 0.894 & 0.089 & 0.069 & 0.056 \\
 & & White & 0.899 & 0.1 & 0.34 & 0.078 & 0.771 & 0.067 & 0.606 & 0.078 \\
 & & Sexual orientation & 0.255 & 0.089 & 0.526 & 0.1 & 0.909 & 0.1 & \cellcolor[HTML]{EA9999}0.007 & \cellcolor[HTML]{F4CCCC}0.033 \\
\cline{2-11}
 & \multirow{9}{*}{Mother-below-bachelor-degree} & First-gen College Student & 0.062 & 0.056 & \cellcolor[HTML]{F4CCCC}0.022 & \cellcolor[HTML]{F4CCCC}0.044 & \cellcolor[HTML]{F4CCCC}0.032 & \cellcolor[HTML]{F4CCCC}0.022 & \cellcolor[HTML]{E06666}0.0 & \cellcolor[HTML]{F4CCCC}0.022 \\
 & & Father's Education & \cellcolor[HTML]{F4CCCC}0.031 & \cellcolor[HTML]{F4CCCC}0.044 & \cellcolor[HTML]{F4CCCC}0.025 & 0.067 & 0.31 & 0.056 & \cellcolor[HTML]{F4CCCC}0.025 & \cellcolor[HTML]{F4CCCC}0.033 \\
 & & Mother's Education & 0.438 & 0.089 & \cellcolor[HTML]{F4CCCC}0.042 & 0.078 & 0.236 & \cellcolor[HTML]{F4CCCC}0.044 & \cellcolor[HTML]{E06666}0.0 & \cellcolor[HTML]{F4CCCC}0.011 \\
 & & Gender & 0.115 & 0.067 & \cellcolor[HTML]{EA9999}0.002 & \cellcolor[HTML]{F4CCCC}0.033 & 0.341 & 0.067 & 0.357 & 0.067 \\
 & & Immigration Status & \cellcolor[HTML]{EA9999}0.003 & \cellcolor[HTML]{F4CCCC}0.022 & \cellcolor[HTML]{E06666}0.0 & \cellcolor[HTML]{F4CCCC}0.022 & 0.591 & 0.089 & 0.298 & 0.056 \\
 & & Asian & \cellcolor[HTML]{F4CCCC}0.01 & \cellcolor[HTML]{F4CCCC}0.033 & \cellcolor[HTML]{F4CCCC}0.023 & 0.056 & 0.713 & 0.1 & 0.395 & 0.078 \\
 & & Biracial & \cellcolor[HTML]{E06666}0.001 & \cellcolor[HTML]{F4CCCC}0.011 & 0.356 & 0.089 & 0.518 & 0.078 & 0.181 & \cellcolor[HTML]{F4CCCC}0.044 \\
 & & White & 0.706 & 0.1 & \cellcolor[HTML]{E06666}0.0 & \cellcolor[HTML]{F4CCCC}0.011 & \cellcolor[HTML]{EA9999}0.006 & \cellcolor[HTML]{F4CCCC}0.011 & 0.423 & 0.089 \\
 & & Sexual orientation & 0.322 & 0.078 & 0.888 & 0.1 & 0.155 & \cellcolor[HTML]{F4CCCC}0.033 & 0.473 & 0.1 \\
\cline{2-11}
 & \multirow{9}{*}{Male} & First-gen College Student & \cellcolor[HTML]{F4CCCC}0.034 & \cellcolor[HTML]{F4CCCC}0.044 & \cellcolor[HTML]{EA9999}0.008 & \cellcolor[HTML]{F4CCCC}0.033 & 0.107 & \cellcolor[HTML]{F4CCCC}0.033 & \cellcolor[HTML]{E06666}0.0 & \cellcolor[HTML]{F4CCCC}0.011 \\
 & & Father's Education & \cellcolor[HTML]{EA9999}0.003 & \cellcolor[HTML]{F4CCCC}0.022 & \cellcolor[HTML]{EA9999}0.003 & \cellcolor[HTML]{F4CCCC}0.022 & 0.65 & 0.089 & 0.093 & 0.067 \\
 & & Mother's Education & 0.112 & 0.078 & 0.576 & 0.1 & 0.123 & \cellcolor[HTML]{F4CCCC}0.044 & \cellcolor[HTML]{E06666}0.001 & \cellcolor[HTML]{F4CCCC}0.022 \\
 & & Gender & 0.063 & 0.056 & \cellcolor[HTML]{E06666}0.0 & \cellcolor[HTML]{F4CCCC}0.011 & 0.36 & 0.056 & \cellcolor[HTML]{F4CCCC}0.039 & \cellcolor[HTML]{F4CCCC}0.044 \\
 & & Immigration Status & 0.087 & 0.067 & \cellcolor[HTML]{F4CCCC}0.014 & \cellcolor[HTML]{F4CCCC}0.044 & 0.469 & 0.078 & 0.489 & 0.078 \\
 & & Asian & \cellcolor[HTML]{F4CCCC}0.015 & \cellcolor[HTML]{F4CCCC}0.033 & 0.203 & 0.067 & \cellcolor[HTML]{F4CCCC}0.02 & \cellcolor[HTML]{F4CCCC}0.011 & 0.784 & 0.1 \\
 & & Biracial & \cellcolor[HTML]{E06666}0.0 & \cellcolor[HTML]{F4CCCC}0.011 & 0.433 & 0.078 & 0.086 & \cellcolor[HTML]{F4CCCC}0.022 & 0.081 & 0.056 \\
 & & White & 0.899 & 0.1 & 0.477 & 0.089 & 0.876 & 0.1 & 0.583 & 0.089 \\
 & & Sexual orientation & 0.255 & 0.089 & 0.188 & 0.056 & 0.374 & 0.067 & \cellcolor[HTML]{EA9999}0.006 & \cellcolor[HTML]{F4CCCC}0.033 \\
\cline{2-11}
 & \multirow{9}{*}{Immigrant} & First-gen College Student & \cellcolor[HTML]{F4CCCC}0.028 & 0.056 & \cellcolor[HTML]{F4CCCC}0.049 & \cellcolor[HTML]{F4CCCC}0.033 & 0.083 & \cellcolor[HTML]{F4CCCC}0.011 & 0.311 & \cellcolor[HTML]{F4CCCC}0.044 \\
 & & Father's Education & \cellcolor[HTML]{F4CCCC}0.025 & \cellcolor[HTML]{F4CCCC}0.044 & \cellcolor[HTML]{F4CCCC}0.035 & \cellcolor[HTML]{F4CCCC}0.011 & 0.484 & 0.056 & 0.941 & 0.1 \\
 & & Mother's Education & 0.399 & 0.078 & 0.112 & 0.078 & 0.111 & \cellcolor[HTML]{F4CCCC}0.022 & 0.478 & 0.056 \\
 & & Gender & \cellcolor[HTML]{F4CCCC}0.041 & 0.067 & 0.439 & 0.1 & 0.239 & \cellcolor[HTML]{F4CCCC}0.033 & \cellcolor[HTML]{F4CCCC}0.011 & \cellcolor[HTML]{F4CCCC}0.011 \\
 & & Immigration Status & \cellcolor[HTML]{E06666}0.0 & \cellcolor[HTML]{F4CCCC}0.011 & 0.051 & \cellcolor[HTML]{F4CCCC}0.044 & 0.815 & 0.078 & 0.592 & 0.067 \\
 & & Asian & \cellcolor[HTML]{EA9999}0.001 & \cellcolor[HTML]{F4CCCC}0.033 & \cellcolor[HTML]{F4CCCC}0.037 & \cellcolor[HTML]{F4CCCC}0.022 & 0.406 & \cellcolor[HTML]{F4CCCC}0.044 & 0.747 & 0.089 \\
 & & Biracial & \cellcolor[HTML]{E06666}0.0 & \cellcolor[HTML]{F4CCCC}0.022 & 0.057 & 0.056 & 0.937 & 0.089 & \cellcolor[HTML]{F4CCCC}0.025 & \cellcolor[HTML]{F4CCCC}0.022 \\
 & & White & 0.424 & 0.089 & 0.068 & 0.067 & 0.806 & 0.067 & 0.068 & \cellcolor[HTML]{F4CCCC}0.033 \\
 & & Sexual orientation & 0.574 & 0.1 & 0.122 & 0.089 & 0.961 & 0.1 & 0.686 & 0.078 \\
\cline{2-11}
 & \multirow{9}{*}{Asian} & First-gen College Student & \cellcolor[HTML]{F4CCCC}0.034 & \cellcolor[HTML]{F4CCCC}0.044 & \cellcolor[HTML]{EA9999}0.009 & \cellcolor[HTML]{F4CCCC}0.022 & 0.404 & 0.056 & \cellcolor[HTML]{E06666}0.0 & \cellcolor[HTML]{F4CCCC}0.011 \\
 & & Father's Education & \cellcolor[HTML]{EA9999}0.003 & \cellcolor[HTML]{F4CCCC}0.022 & \cellcolor[HTML]{F4CCCC}0.032 & \cellcolor[HTML]{F4CCCC}0.033 & 0.621 & 0.078 & 0.072 & 0.067 \\
 & & Mother's Education & 0.112 & 0.078 & 0.711 & 0.1 & 0.379 & \cellcolor[HTML]{F4CCCC}0.044 & \cellcolor[HTML]{E06666}0.001 & \cellcolor[HTML]{F4CCCC}0.022 \\
 & & Gender & 0.063 & 0.056 & 0.09 & 0.056 & 0.341 & \cellcolor[HTML]{F4CCCC}0.033 & \cellcolor[HTML]{F4CCCC}0.031 & \cellcolor[HTML]{F4CCCC}0.044 \\
 & & Immigration Status & 0.087 & 0.067 & \cellcolor[HTML]{E06666}0.001 & \cellcolor[HTML]{F4CCCC}0.011 & 0.838 & 0.1 & 0.631 & 0.089 \\
 & & Asian & \cellcolor[HTML]{F4CCCC}0.015 & \cellcolor[HTML]{F4CCCC}0.033 & 0.118 & 0.067 & \cellcolor[HTML]{F4CCCC}0.02 & \cellcolor[HTML]{F4CCCC}0.011 & 0.945 & 0.1 \\
 & & Biracial & \cellcolor[HTML]{E06666}0.0 & \cellcolor[HTML]{F4CCCC}0.011 & 0.089 & \cellcolor[HTML]{F4CCCC}0.044 & 0.107 & \cellcolor[HTML]{F4CCCC}0.022 & 0.069 & 0.056 \\
 & & White & 0.899 & 0.1 & 0.286 & 0.078 & 0.547 & 0.067 & 0.606 & 0.078 \\
 & & Sexual orientation & 0.255 & 0.089 & 0.491 & 0.089 & 0.836 & 0.089 & \cellcolor[HTML]{EA9999}0.007 & \cellcolor[HTML]{F4CCCC}0.033 \\
\cline{2-11}
 & \multirow{9}{*}{Biracial} & First-gen College Student & \cellcolor[HTML]{F4CCCC}0.034 & \cellcolor[HTML]{F4CCCC}0.044 & \cellcolor[HTML]{E06666}0.0 & \cellcolor[HTML]{F4CCCC}0.011 & 0.18 & \cellcolor[HTML]{F4CCCC}0.022 & \cellcolor[HTML]{E06666}0.0 & \cellcolor[HTML]{F4CCCC}0.011 \\
 & & Father's Education & \cellcolor[HTML]{EA9999}0.003 & \cellcolor[HTML]{F4CCCC}0.022 & \cellcolor[HTML]{E06666}0.0 & \cellcolor[HTML]{F4CCCC}0.022 & 0.777 & 0.089 & 0.072 & 0.067 \\
 & & Mother's Education & 0.112 & 0.078 & 0.19 & 0.056 & 0.273 & \cellcolor[HTML]{F4CCCC}0.033 & \cellcolor[HTML]{E06666}0.001 & \cellcolor[HTML]{F4CCCC}0.022 \\
 & & Gender & 0.063 & 0.056 & \cellcolor[HTML]{EA9999}0.01 & \cellcolor[HTML]{F4CCCC}0.044 & 0.418 & 0.056 & \cellcolor[HTML]{F4CCCC}0.031 & \cellcolor[HTML]{F4CCCC}0.044 \\
 & & Immigration Status & 0.087 & 0.067 & \cellcolor[HTML]{EA9999}0.005 & \cellcolor[HTML]{F4CCCC}0.033 & 0.952 & 0.1 & 0.631 & 0.089 \\
 & & Asian & \cellcolor[HTML]{F4CCCC}0.015 & \cellcolor[HTML]{F4CCCC}0.033 & 0.917 & 0.1 & \cellcolor[HTML]{F4CCCC}0.044 & \cellcolor[HTML]{F4CCCC}0.011 & 0.945 & 0.1 \\
 & & Biracial & \cellcolor[HTML]{E06666}0.0 & \cellcolor[HTML]{F4CCCC}0.011 & 0.657 & 0.089 & 0.274 & \cellcolor[HTML]{F4CCCC}0.044 & 0.069 & 0.056 \\
 & & White & 0.899 & 0.1 & 0.448 & 0.078 & 0.672 & 0.067 & 0.606 & 0.078 \\
 & & Sexual orientation & 0.255 & 0.089 & 0.222 & 0.067 & 0.76 & 0.078 & \cellcolor[HTML]{EA9999}0.007 & \cellcolor[HTML]{F4CCCC}0.033 \\
\cline{2-11}
 & \multirow{9}{*}{White} & First-gen College Student & \cellcolor[HTML]{F4CCCC}0.034 & \cellcolor[HTML]{F4CCCC}0.044 & \cellcolor[HTML]{EA9999}0.001 & \cellcolor[HTML]{F4CCCC}0.022 & 0.198 & \cellcolor[HTML]{F4CCCC}0.022 & \cellcolor[HTML]{E06666}0.0 & \cellcolor[HTML]{F4CCCC}0.011 \\
 & & Father's Education & \cellcolor[HTML]{EA9999}0.003 & \cellcolor[HTML]{F4CCCC}0.022 & \cellcolor[HTML]{F4CCCC}0.013 & \cellcolor[HTML]{F4CCCC}0.044 & 0.454 & 0.056 & 0.072 & 0.067 \\
 & & Mother's Education & 0.112 & 0.078 & 0.282 & 0.056 & 0.216 & \cellcolor[HTML]{F4CCCC}0.033 & \cellcolor[HTML]{E06666}0.001 & \cellcolor[HTML]{F4CCCC}0.022 \\
 & & Gender & 0.063 & 0.056 & \cellcolor[HTML]{E06666}0.0 & \cellcolor[HTML]{F4CCCC}0.011 & 0.36 & \cellcolor[HTML]{F4CCCC}0.044 & \cellcolor[HTML]{F4CCCC}0.031 & \cellcolor[HTML]{F4CCCC}0.044 \\
 & & Immigration Status & 0.087 & 0.067 & \cellcolor[HTML]{EA9999}0.005 & \cellcolor[HTML]{F4CCCC}0.033 & 0.701 & 0.067 & 0.631 & 0.089 \\
 & & Asian & \cellcolor[HTML]{F4CCCC}0.015 & \cellcolor[HTML]{F4CCCC}0.033 & 0.591 & 0.078 & 0.154 & \cellcolor[HTML]{F4CCCC}0.011 & 0.945 & 0.1 \\
 & & Biracial & \cellcolor[HTML]{E06666}0.0 & \cellcolor[HTML]{F4CCCC}0.011 & 0.953 & 0.1 & 0.904 & 0.089 & 0.069 & 0.056 \\
 & & White & 0.899 & 0.1 & 0.3 & 0.067 & 0.876 & 0.078 & 0.606 & 0.078 \\
 & & Sexual orientation & 0.255 & 0.089 & 0.94 & 0.089 & 0.94 & 0.1 & \cellcolor[HTML]{EA9999}0.007 & \cellcolor[HTML]{F4CCCC}0.033 \\
\cline{2-11}
 & \multirow{9}{*}{Non-heterosexual} & First-gen College Student & \cellcolor[HTML]{F4CCCC}0.028 & 0.056 & \cellcolor[HTML]{E06666}0.0 & \cellcolor[HTML]{F4CCCC}0.011 & 0.18 & \cellcolor[HTML]{F4CCCC}0.033 & \cellcolor[HTML]{F4CCCC}0.024 & \cellcolor[HTML]{F4CCCC}0.022 \\
 & & Father's Education & \cellcolor[HTML]{F4CCCC}0.01 & \cellcolor[HTML]{F4CCCC}0.033 & \cellcolor[HTML]{EA9999}0.002 & \cellcolor[HTML]{F4CCCC}0.022 & 0.991 & 0.1 & 0.081 & 0.056 \\
 & & Mother's Education & 0.09 & 0.078 & \cellcolor[HTML]{F4CCCC}0.043 & 0.056 & 0.273 & \cellcolor[HTML]{F4CCCC}0.044 & 0.209 & 0.089 \\
 & & Gender & \cellcolor[HTML]{F4CCCC}0.041 & 0.067 & \cellcolor[HTML]{F4CCCC}0.022 & \cellcolor[HTML]{F4CCCC}0.033 & 0.418 & 0.056 & 0.122 & 0.067 \\
 & & Immigration Status & \cellcolor[HTML]{F4CCCC}0.017 & \cellcolor[HTML]{F4CCCC}0.044 & \cellcolor[HTML]{F4CCCC}0.024 & \cellcolor[HTML]{F4CCCC}0.044 & 0.67 & 0.078 & \cellcolor[HTML]{F4CCCC}0.027 & \cellcolor[HTML]{F4CCCC}0.033 \\
 & & Asian & \cellcolor[HTML]{EA9999}0.005 & \cellcolor[HTML]{F4CCCC}0.022 & 0.149 & 0.078 & \cellcolor[HTML]{F4CCCC}0.021 & \cellcolor[HTML]{F4CCCC}0.011 & 0.075 & \cellcolor[HTML]{F4CCCC}0.044 \\
 & & Biracial & \cellcolor[HTML]{E06666}0.0 & \cellcolor[HTML]{F4CCCC}0.011 & 0.133 & 0.067 & 0.159 & \cellcolor[HTML]{F4CCCC}0.022 & 0.154 & 0.078 \\
 & & White & 0.583 & 0.1 & 0.452 & 0.1 & 0.672 & 0.089 & 0.545 & 0.1 \\
 & & Sexual orientation & 0.415 & 0.089 & 0.275 & 0.089 & 0.622 & 0.067 & \cellcolor[HTML]{E06666}0.0 & \cellcolor[HTML]{F4CCCC}0.011 \\
\cline{2-11}
\hline

\end{tabular}}
\caption{}\label{tab:acc_demo2_appendix}
\end{table}
