# Supplementary material for: A Framework for Designing Fair Ubiquitous Computing Systems
Source: arXiv:2308.08710 source file (2023-08-17)
Supplement: Supplementary file 4 [file tab_fpr_w_t_demo_appendix.tex]

\begin{table}[htb!]

   \resizebox{0.8\textwidth}{!}{\begin{tabular}{|l|l|rr|rr|rr|rr|}\hline
&& \multicolumn{2}{c|}{\cellcolor[HTML]{CCCCCC}\textbf{DS1 (2018)}}        & \multicolumn{2}{c|}{\cellcolor[HTML]{CCCCCC}\textbf{DS2 (2019)}}        & \multicolumn{2}{c|}{\cellcolor[HTML]{CCCCCC}\textbf{DS3 (2020)}}        & \multicolumn{2}{c|}{\cellcolor[HTML]{CCCCCC}\textbf{DS4 (2021)}}        \\\cline{3-10}
\multirow{-2}{*}{}& \multirow{-2}{*}{\textbf{Sensitive Sub-attributes}} & \multicolumn{1}{c}{p values}  & \multicolumn{1}{c|}{q values}  & \multicolumn{1}{c}{p values}  & \multicolumn{1}{c|}{q values}  & \multicolumn{1}{c}{p values}  & \multicolumn{1}{c|}{q values}  & \multicolumn{1}{c}{p values}  & \multicolumn{1}{c|}{q values}  \\\hline
    & First-gen College Student              & 1.000& 0.056& \cellcolor[HTML]{E06666}0.000 & \cellcolor[HTML]{F4CCCC}0.011 & 0.146& 0.044& \cellcolor[HTML]{F4CCCC}0.031 & \cellcolor[HTML]{F4CCCC}0.033 \\
    & Father's Education & 1.000& 0.056& 0.414& 0.078& 0.440& 0.078& \cellcolor[HTML]{E06666}0.001 & \cellcolor[HTML]{F4CCCC}0.011 \\
    & Mother's Education & 1.000& 0.056& \cellcolor[HTML]{F4CCCC}0.011 & \cellcolor[HTML]{F4CCCC}0.033 & 0.214& 0.056& \cellcolor[HTML]{F4CCCC}0.023 & 0.022\\
    & Gender        & 1.000& 0.056& 0.166& 0.067& 0.053& 0.033& 0.084& 0.056\\
    & Immigration Status & 1.000& 0.056& \cellcolor[HTML]{EA9999}0.007 & \cellcolor[HTML]{F4CCCC}0.022 & 0.741& 0.100& 0.626& 0.089\\
    & Asian         & 1.000& 0.056& 0.861& 0.089& 0.347& 0.067& 0.706& 0.100\\
    & Biracial      & 1.000& 0.056& 0.134& 0.056& \cellcolor[HTML]{E06666}0.000 & \cellcolor[HTML]{F4CCCC}0.022 & 0.367& 0.067\\
    & White         & 1.000& 0.056& 0.104& 0.044& \cellcolor[HTML]{E06666}0.000 & \cellcolor[HTML]{F4CCCC}0.011 & 0.062& 0.044\\
\multirow{-9}{*}{Wahle \etal \cite{wahle2016mobile}}               & Sexual Orientation & 1.000& 0.056& 0.984& 0.100& 0.606& 0.089& 0.489& 0.078\\ \hline
    & First-gen College Student              & 0.260& 0.078& 1.000& 0.056& \cellcolor[HTML]{F4CCCC}0.014 & \cellcolor[HTML]{F4CCCC}0.033 & 0.348& 0.044\\
    & Father's Education & 0.054& 0.033& 1.000& 0.056& 0.528& 0.067& 0.664& 0.078\\
    & Mother's Education & \cellcolor[HTML]{F4CCCC}0.032 & 0.011& 1.000& 0.056& 0.973& 0.100& 0.672& 0.100\\
    & Gender        & 0.062& 0.044& 1.000& 0.056& 0.372& 0.056& 0.668& 0.089\\
    & Immigration Status & 0.276& 0.089& 1.000& 0.056& 0.550& 0.078& 0.563& 0.067\\
    & Asian         & 0.089& 0.067& 1.000& 0.056& 0.206& 0.044& \cellcolor[HTML]{F4CCCC}0.028 & 0.022\\
    & Biracial      & 0.076& 0.056& 1.000& 0.056& \cellcolor[HTML]{EA9999}0.008 & \cellcolor[HTML]{F4CCCC}0.022 & 0.135& 0.033\\
    & White         & \cellcolor[HTML]{F4CCCC}0.050 & 0.022& 1.000& 0.056& \cellcolor[HTML]{EA9999}0.002 & \cellcolor[HTML]{F4CCCC}0.011 & \cellcolor[HTML]{F4CCCC}0.015 & 0.011\\
\multirow{-9}{*}{Saeb \etal \cite{saeb2015mobile}}                 & Sexual Orientation & 0.792& 0.100& 1.000& 0.056& 0.821& 0.089& 0.460& 0.056\\ \hline
%     & First-gen College Student              & 0.219& 0.033& \cellcolor[HTML]{F4CCCC}0.018 & 0.011& 0.892& 0.100& 0.085& 0.033\\
%     & Father's Education & 0.939& 0.100& 0.218& 0.022& \cellcolor[HTML]{EA9999}0.010 & \cellcolor[HTML]{F4CCCC}0.022 & \cellcolor[HTML]{F4CCCC}0.038 & 0.022\\
%     & Mother's Education & 0.246& 0.044& 0.646& 0.067& 0.370& 0.067& \cellcolor[HTML]{F4CCCC}0.022 & 0.011\\
%     & Gender        & 0.334& 0.078& 0.571& 0.056& 0.348& 0.044& 0.346& 0.067\\
%     & Immigration Status & 0.620& 0.089& 0.646& 0.078& 0.600& 0.078& 0.423& 0.078\\
%     & Asian         & 0.067& 0.022& 0.484& 0.044& 0.362& 0.056& 0.635& 0.089\\
%     & Biracial      & 0.272& 0.067& 0.402& 0.033& \cellcolor[HTML]{F4CCCC}0.027 & \cellcolor[HTML]{F4CCCC}0.033 & 0.133& 0.056\\
%     & White         & \cellcolor[HTML]{F4CCCC}0.042 & 0.011& 0.707& 0.089& \cellcolor[HTML]{EA9999}0.010 & \cellcolor[HTML]{F4CCCC}0.011 & 0.112& 0.044\\
% \multirow{-9}{*}{Farhan \etal \cite{farhan2016behavior}}           & Sexual Orientation & 0.260& 0.056& 0.929& 0.100& 0.784& 0.089& 0.945& 0.100\\ \hline
    & First-gen College Student              & 1.000& 0.056& 0.066& 0.056& 0.481& 0.033& 0.972& 0.100\\
    & Father's Education & 1.000& 0.056& 0.260& 0.078& 0.243& 0.022& 0.546& 0.067\\
    & Mother's Education & 1.000& 0.056& \cellcolor[HTML]{EA9999}0.003 & \cellcolor[HTML]{F4CCCC}0.022 & 0.726& 0.078& \cellcolor[HTML]{F4CCCC}0.037 & 0.033\\
    & Gender        & 1.000& 0.056& \cellcolor[HTML]{F4CCCC}0.024 & \cellcolor[HTML]{F4CCCC}0.033 & 0.582& 0.044& \cellcolor[HTML]{EA9999}0.003 & \cellcolor[HTML]{F4CCCC}0.011 \\
    & Immigration Status & 1.000& 0.056& \cellcolor[HTML]{EA9999}0.001 & \cellcolor[HTML]{F4CCCC}0.011 & \cellcolor[HTML]{F4CCCC}0.012 & 0.011& 0.511& 0.056\\
    & Asian         & 1.000& 0.056& 0.893& 0.100& 0.726& 0.078& \cellcolor[HTML]{F4CCCC}0.045 & 0.044\\
    & Biracial      & 1.000& 0.056& 0.075& 0.067& 0.646& 0.067& 0.962& 0.089\\
    & White         & 1.000& 0.056& 0.063& 0.044& 0.622& 0.056& \cellcolor[HTML]{F4CCCC}0.030 & 0.022\\
\multirow{-9}{*}{Canzian \etal \cite{canzian2015trajectories}}     & Sexual Orientation & 1.000& 0.056& 0.542& 0.089& 0.861& 0.100& 0.547& 0.078\\ \hline
    & First-gen College Student              & 0.548& 0.044& 0.083& 0.044& 0.704& 0.089& 0.207& 0.044\\
    & Father's Education & 0.929& 0.089& 0.082& 0.033& \cellcolor[HTML]{E06666}0.000 & \cellcolor[HTML]{F4CCCC}0.011 & 0.536& 0.078\\
    & Mother's Education & 0.549& 0.056& 0.277& 0.089& 0.605& 0.078& 0.298& 0.056\\
    & Gender        & 0.688& 0.067& \cellcolor[HTML]{F4CCCC}0.043 & 0.022& 0.488& 0.056& 0.537& 0.089\\
    & Immigration Status & 0.383& 0.033& \cellcolor[HTML]{F4CCCC}0.018 & 0.011& 0.757& 0.100& 0.426& 0.067\\
    & Asian         & 0.708& 0.078& 0.185& 0.078& \cellcolor[HTML]{F4CCCC}0.040 & 0.022& \cellcolor[HTML]{EA9999}0.008 & \cellcolor[HTML]{F4CCCC}0.011 \\
    & Biracial      & \cellcolor[HTML]{F4CCCC}0.019 & 0.011& 0.086& 0.056& 0.109& 0.044& 0.094& 0.022\\
    & White         & 0.071& 0.022& 0.151& 0.067& 0.082& 0.033& 0.560& 0.100\\
\multirow{-9}{*}{Wang \etal \cite{wang2018tracking}}               & Sexual Orientation & 0.998& 0.100& 0.988& 0.100& 0.574& 0.067& 0.113& 0.033\\ \hline
%     & First-gen College Student              & 0.257& 0.044& 1.000& 0.056& 0.100& 0.022& 0.372& 0.067\\
%     & Father's Education & 0.618& 0.078& 1.000& 0.056& \cellcolor[HTML]{F4CCCC}0.029 & 0.011& \cellcolor[HTML]{E06666}0.000 & \cellcolor[HTML]{F4CCCC}0.011 \\
%     & Mother's Education & 0.324& 0.056& 1.000& 0.056& 0.556& 0.100& 0.367& 0.056\\
%     & Gender        & 0.915& 0.100& 1.000& 0.056& 0.183& 0.044& 0.784& 0.089\\
%     & Immigration Status & 0.798& 0.089& 1.000& 0.056& 0.426& 0.078& 0.154& 0.033\\
%     & Asian         & \cellcolor[HTML]{F4CCCC}0.019 & \cellcolor[HTML]{F4CCCC}0.022 & 1.000& 0.056& 0.103& 0.033& 0.920& 0.100\\
%     & Biracial      & \cellcolor[HTML]{EA9999}0.005 & \cellcolor[HTML]{F4CCCC}0.011 & 1.000& 0.056& 0.292& 0.067& 0.156& 0.044\\
%     & White         & 0.059& 0.033& 1.000& 0.056& 0.259& 0.056& 0.124& 0.022\\
% \multirow{-9}{*}{Lu etal \cite{lu2018joint}}             & Sexual Orientation & 0.541& 0.067& 1.000& 0.056& 0.451& 0.089& 0.569& 0.078\\ \hline
    & First-gen College Student              & 0.969& 0.089& 0.143& 0.044& 0.790& 0.089& 0.063& 0.011\\
    & Father's Education & 0.460& 0.056& 0.819& 0.100& 0.835& 0.100& 0.199& 0.022\\
    & Mother's Education & 0.996& 0.100& 0.068& 0.033& 0.290& 0.056& 0.524& 0.033\\
    & Gender        & 0.320& 0.044& \cellcolor[HTML]{F4CCCC}0.024 & 0.022& 0.132& 0.033& 0.651& 0.056\\
    & Immigration Status & 0.743& 0.067& 0.156& 0.056& 0.059& 0.011& 0.764& 0.078\\
    & Asian         & 0.139& 0.033& 0.195& 0.067& 0.780& 0.078& 0.651& 0.044\\
    & Biracial      & 0.791& 0.078& 0.236& 0.078& 0.112& 0.022& 0.783& 0.089\\
    & White         & 0.130& 0.022& 0.657& 0.089& 0.228& 0.044& 0.790& 0.100\\
\multirow{-9}{*}{Xu \etal - Interpretable \cite{xu2019leveraging}} & Sexual Orientation & \cellcolor[HTML]{F4CCCC}0.017 & 0.011& \cellcolor[HTML]{F4CCCC}0.015 & 0.011& 0.398& 0.067& 0.705& 0.067\\ \hline
    & First-gen College Student              & 0.853& 0.089& 0.310& 0.067& 0.069& 0.011& 0.182& 0.044\\
    & Father's Education & 0.211& 0.033& 0.861& 0.089& 0.833& 0.089& 0.723& 0.078\\
    & Mother's Education & 0.212& 0.044& 0.537& 0.078& 0.609& 0.067& 0.178& 0.033\\
    & Gender        & 0.456& 0.067& 0.221& 0.056& 0.466& 0.056& 0.982& 0.100\\
    & Immigration Status & 0.249& 0.056& 0.143& 0.044& 0.317& 0.044& 0.940& 0.089\\
    & Asian         & 0.941& 0.100& \cellcolor[HTML]{F4CCCC}0.045 & 0.033& 0.609& 0.067& 0.342& 0.056\\
    & Biracial      & 0.076& 0.011& 0.996& 0.100& 0.157& 0.033& \cellcolor[HTML]{F4CCCC}0.036 & 0.022\\
    & White         & 0.501& 0.078& \cellcolor[HTML]{EA9999}0.010 & \cellcolor[HTML]{F4CCCC}0.022 & 0.881& 0.100& 0.682& 0.067\\
\multirow{-9}{*}{Xu \etal - Personalized \cite{xu2022survey}}      & Sexual Orientation & 0.130& 0.022& \cellcolor[HTML]{E06666}0.000 & \cellcolor[HTML]{F4CCCC}0.011 & 0.155& 0.022& \cellcolor[HTML]{EA9999}0.010 & \cellcolor[HTML]{F4CCCC}0.011 \\\hline 
    & First-gen College Student              & 0.725& 0.089& 0.654& 0.078& 0.420& 0.067& \cellcolor[HTML]{EA9999}0.002 & \cellcolor[HTML]{F4CCCC}0.011 \\
    & Father's Education & 0.593& 0.067& 0.910& 0.100& 0.921& 0.100& 0.217& 0.044\\
    & Mother's Education & 0.483& 0.056& 0.197& 0.056& 0.311& 0.044& 0.537& 0.078\\
    & Gender        & 0.416& 0.033& \cellcolor[HTML]{F4CCCC}0.050 & 0.033& 0.557& 0.078& 0.653& 0.089\\
    & Immigration Status & 0.467& 0.044& 0.846& 0.089& 0.327& 0.056& 0.899& 0.100\\
    & Asian         & 0.600& 0.078& 0.326& 0.067& \cellcolor[HTML]{F4CCCC}0.022 & 0.011& 0.455& 0.067\\
    & Biracial      & 0.993& 0.100& \cellcolor[HTML]{F4CCCC}0.024 & 0.011& 0.103& 0.033& \cellcolor[HTML]{F4CCCC}0.023 & \cellcolor[HTML]{F4CCCC}0.033 \\
    & White         & 0.388& 0.022& 0.139& 0.044& \cellcolor[HTML]{F4CCCC}0.030 & 0.022& \cellcolor[HTML]{F4CCCC}0.011 & \cellcolor[HTML]{F4CCCC}0.022 \\
\multirow{-9}{*}{Chikersal \etal \cite{chikersal2021detecting}}    & Sexual Orientation & 0.285& 0.011& \cellcolor[HTML]{F4CCCC}0.045 & 0.022& 0.654& 0.089& 0.376& 0.056\\ \hline
\end{tabular}}\label{tab_fpr_w_t_demo_appendix}
\caption{FPR.}
\end{table}
